# Supplementary material for: Interfacial free energy of a hard-sphere fluid in contact with curved hard surfaces
Source: arXiv:1209.5383 source file (2012-09-24)
Supplement: Supplementary file 1 [file Laird-Hunter-Davidchack_supplemental.pdf]

**Supplemental Information for "Curvature dependance of the interfacial free energy of a hard-sphere fluid at a hard wall"**

Brian B. Laird*[1], Allie Hunter[1] and Ruslan L. Davidchack[2]

[1] *Department of Chemistry, University of Kansas, Lawrence, KS 66045, USA*

[2] *Department of Mathematics, University of Leicester, Leicester, LE1 7RH, UK*

**Table of Contents**

- **S1:** Additional Simulation Details
- **S2:** Results for $v_N$ for a hard-sphere fluid at spherical and cylindrical hard walls.
- **S3:** Results from the weighed least-squares fits for the calculation of $h$ and $\kappa$

**Section S1: Additional Simulation Details**:

For the simulations involving a spherical wall, the simulation cell is a cube with side $L$ containing $N_{\text{total}}$ spheres. Periodic boundary conditions are applied in all directions. A spherical wall of radius $R$ is placed in the middle of the cube. The volume of the system is thus $V_{\text{total}} = L^3 - \frac{4}{3}\pi R^3$. We then define $V(r)$ as volume outside $R$ and inside $r$, that is, $V(r) = \frac{4}{3}\pi(r^3 - R^3)$, and measure the average number of spheres inside this volume, $N(r)$, during a molecular dynamics simulation run. If $r$ is sufficiently large (but smaller than $L/2$), then we can assume that the system properties outside $r$ are those of the bulk fluid and thus take $V_f = V_{\text{total}} - V(r)$ and $N_f = N_{\text{total}} - N(r)$. Eq. 6 in the paper then becomes:

$$v(r) = \frac{1}{A}\left[V(r) - \frac{V_{\text{total}} - V(r)}{N_{\text{total}} - N(r)} N(r)\right], \quad (1)$$

where $A = 4\pi R^2$. To determine the excess interfacial volume, we calculate $v(r)$ for increasing values of $r$ and find a place where $v(r)$ stops oscillating and reaches a plateau. The value of $v(r)$ at this plateau is taken to be the excess interfacial volume. For the cylindrical wall with radius $R$ and length $L_z$, we use the simulation cell with dimensions $L$ by $L$ by $L_z$ with the wall axis parallel to $z$. Then $V_{\text{total}} = (L^2 - \pi R^2)L_z$, $V(r) = \pi(r^2 - R^2)L_z$, and $A = 2\pi R L_z$.

The values of $L$ range from $14\,\sigma$ for systems with small $R$ and low density to $56\,\sigma$ for systems with large $R$ and high density. We use $L_z = 20\,\sigma$ for all systems with the cylindrical wall.

**Section S2: Results for $v_N$ for a hard-sphere fluid at spherical and cylindrical hard walls:**

Fig. S1 shows the values of the excess interfacial volume as a function of packing fraction, $\eta$, for the hard-sphere fluid for spherical and cylindrical walls for several values of the wall radius $R$.

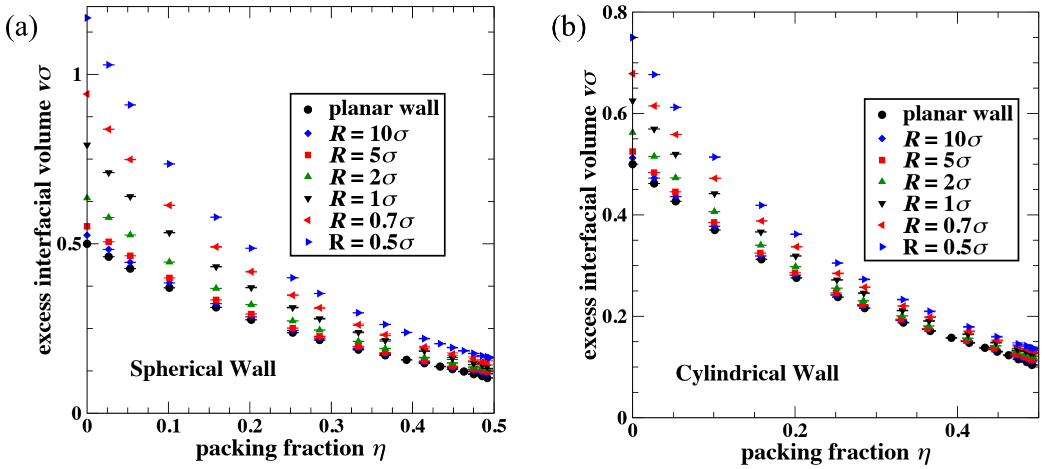


FIG. S1 . (a) Excess interfacial volume, $v_{ex}$, for the hard-sphere fluid at a spherical wall at a function of $\eta$ for several values of sphere radius, $R$. (b) Same as in (a) for a cylindrical wall, where $R$ is the cylinder radius.

Fig. S2 shows the data for $v_{ex}$ shown in Fig. S1 for the hard-sphere fluid at a spherical wall, but restricted to packing fractions between 0.4 and 0.5.

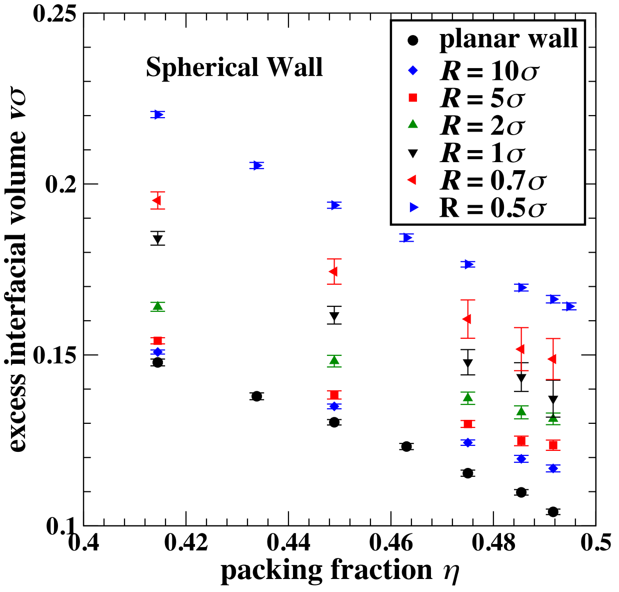


FIG. S2 . Excess interfacial volume, $v_{ex}$, for the hard-sphere fluid at a spherical wall at a function of packing fraction $\eta$ for several values of sphere radius, $R$ in the range $0.4 < \eta < 0.5$.

TABLE S1 . Fitting coefficients for the hard-sphere fluid at a hard spherical or cylindrical colloidal particle from the weighted least-squares regression fit to Eq. 1 in the text. The numbers in parentheses show the 95% confidence level uncertainties in the lasts digits shown. The values for $\gamma_0$ shown are those corresponding to the spherical particle, which are identical within the error bars to the corresponding quantity for the cylindrical particle and to the data for the planar wall given in Ref. 11.

| $\eta$ | $\gamma_0\sigma^2/kT$ | $h_s\sigma/kT$ | $\kappa_s/kT$ | $h_c\sigma/kT$ | $\gamma_0^{\mathrm{SPT}}\sigma^2/kT$ | $h_{\mathrm{SPT}}\sigma/kT$ | $\kappa_{\mathrm{SPT}}/kT$ |
|---|---|---|---|---|---|---|---|
| 0 | 0 | 0 | 0 | 0 | 0 | 0 | 0 |
| 0.02656 | 0.027105(5) | 0.013025(18) | 0.002147(10) | 0.013072(4) | 0.027116 | 0.013027 | 0.002142 |
| 0.05306 | 0.057923(12) | 0.02679(4) | 0.00434(2) | 0.026928(18) | 0.057999 | 0.02675 | 0.004338 |
| 0.10116 | 0.12499(3) | 0.05396(11) | 0.00848(6) | 0.05444(6) | 0.125612 | 0.05374 | 0.008487 |
| 0.15860 | 0.22805(8) | 0.0909(3) | 0.01368(16) | 0.091618(14) | 0.23089 | 0.09000 | 0.01374 |
| 0.20172 | 0.32624(14) | 0.1223(5) | 0.0178(3) | 0.1238(4) | 0.33277 | 0.12065 | 0.01793 |
| 0.25265 | 0.4715(2) | 0.1650(9) | 0.0229(4) | 0.1668(4) | 0.48651 | 0.16141 | 0.02317 |
| 0.28568 | 0.5870 (4) | 0.1969(13) | 0.0263(6) | 0.1984(6) | 0.61104 | 0.19095 | 0.02677 |
| 0.33335 | 0.7906(6) | 0.248(2) | 0.0263(6) | 0.2496(8) | 0.83568 | 0.2388 | 0.03227 |
| 0.36636 | 0.9640(9) | 0.289(3) | 0.0346(14) | 0.2902(12) | 1.03094 | 0.2761 | 0.03631 |
| 0.41449 | 1.2783(13) | 0.358(5) | 0.040(3) | 0.3600(18) | 1.39379 | 0.3380 | 0.04260 |

**Section S3: Results from the weighed least-squares fits for the calculation of $h$ and $\kappa$:**

Table S1 shows the values of the fitting coefficients $\gamma_0$, $h$ and $\kappa$ defined in Eq. 1 of the paper that were determined from the simulation results using weighted least-squares regression. In addition, the values of the corresponding parameters from SPT are given at each packing fraction.
